# Supplementary material for: Mitigating Object Hallucinations in Large Vision-Language Models through Visual Contrastive Decoding
Source: arXiv:2311.16922 source file (2023-11-28)
Supplement: Supplementary file 1 [file _supplementary.tex]

% \input{_constants}
% \review % \review OR \cameraready

% \documentclass[10pt,twocolumn,letterpaper]{article}
% \input{cvpr_header}
% \myexternaldocument{_main}
% \begin{document}

% %% TITLE
% \title{\paperTitle}
% \author{\authorBlock}
% \maketitlesupplementary
% %%

% \input{12_appendix}

% {\small
% \bibliographystyle{ieeenat_fullname}
% \bibliography{11_references}
% }

% \end{document}
